# Supplementary material for: Mindalogue: LLM-Powered Nonlinear Interaction for Effective Learning and Task Exploration
Source: arXiv:2410.10570 source file (2024-10-15)
Supplement: Supplementary file 1 [file 13_supplementary.tex]

\appendix

% In the supplementary material, two sections are provided: the experimental conditions and the user questionnaire from the evaluation study.

\section{EXPERIMENTAL CONDITION}

As shown in Table \ref{tab:Experimental Condition Setting}, 16 participants were assigned different topics sequentially and completed two tasks on two systems for comparison. Each participant completed tasks in all four task categories. To ensure balance, there were 16 samples for each task category, resulting in 32 samples for each system. S1 refers to System 1 (Mindalogue), while S2 refers to System 2 (Mindmap Master).

\begin{table*}[htbp]
  \caption{Experimental Condition Setting}
  \label{tab:Experimental Condition Setting}
  %\scriptsize
  \resizebox{\textwidth}{!}{
    \begin{tabular}{lllllllllllllllllllll}
      \toprule
      Task Category & \multicolumn{8}{l}{C1: Knowledge Exploration} & \multicolumn{8}{l}{C2: Brainstorming} & \multicolumn{2}{l}{C3: Product Analysis} & \multicolumn{2}{l}{C4: City Description} \\
      \midrule
      Topic & \multicolumn{2}{l}{\begin{tabular}[c]{@{}l@{}}T1\\ Machine\\ Learning\end{tabular}} & \multicolumn{2}{l}{\begin{tabular}[c]{@{}l@{}}T2\\ Dadaism\end{tabular}} & \multicolumn{2}{l}{\begin{tabular}[c]{@{}l@{}}T3\\ Relativity\end{tabular}} & \multicolumn{2}{l}{\begin{tabular}[c]{@{}l@{}}T4\\ Industrial Revolution\end{tabular}} & \multicolumn{2}{l}{\begin{tabular}[c]{@{}l@{}}T5\\ Future fashion design\end{tabular}} & \multicolumn{2}{l}{\begin{tabular}[c]{@{}l@{}}T6\\ Commercial dream experience\end{tabular}} & \multicolumn{2}{l}{\begin{tabular}[c]{@{}l@{}}T7\\ Digital food design\end{tabular}} & \multicolumn{2}{l}{\begin{tabular}[c]{@{}l@{}}T8\\ Event planning without digital products\end{tabular}} & \multicolumn{2}{l}{\begin{tabular}[c]{@{}l@{}}T9\\ Recommend a commonly used mobile app\end{tabular}} & \multicolumn{2}{l}{\begin{tabular}[c]{@{}l@{}}T10\\ Recommend a city\\ (e.g., a favorite city, hometown)\end{tabular}} \\
      \midrule
      P1  & T1S1 &       &       &       &       &       &       &       &       & T5S2 &       &       &       &       &       &       & T9S1 &       &       & T10S2 \\
      P2  &      & T1S2  &       &       &       &       &       &       &       &      & T6S1 &       &       &       &       &       &      & T9S2 & T10S1 &        \\
      P3  &      &       & T2S1  &       &       &       &       &       &       &      &      & T6S2 &       &       &       &       & T9S1 &       &       & T10S2 \\
      P4  &      &       &       & T2S2  &       &       &       &       &       &      &      &      & T7S1  &       &       &       &      & T9S2 & T10S1 &        \\
      P5  &      &       &       &       & T3S1  &       &       &       &       &      &      &      &       & T7S2  &       &       & T9S1 &       &       & T10S2 \\
      P6  &      &       &       &       &       & T3S2  &       &       &       &      &      &      &       &       & T8S1  &       &      & T9S2 & T10S1 &        \\
      P7  &      &       &       &       &       &       & T4S1  &       &       &      &      &      &       &       &       & T8S2  & T9S1 &       &       & T10S2 \\
      P8  &      &       &       &       &       &       &       & T4S2  & T5S1  &      &      &      &       &       &       &       &      & T9S2 & T10S1 &        \\
      P9  & T1S1 &       &       &       &       &       &       &       &       & T5S2 &      &      &       &       &       &       & T9S1 &       &       & T10S2 \\
      P10 &      & T1S2  &       &       &       &       &       &       &       &      & T6S1 &      &       &       &       &       &      & T9S2 & T10S1 &        \\
      P11 &      &       & T2S1  &       &       &       &       &       &       &      &      & T6S2 &       &       &       &       & T9S1 &       &       & T10S2 \\
      P12 &      &       &       & T2S2  &       &       &       &       &       &      &      &      & T7S1  &       &       &       &      & T9S2 & T10S1 &        \\
      P13 &      &       &       &       & T3S1  &       &       &       &       &      &      &      &       & T7S2  &       &       & T9S1 &       &       & T10S2 \\
      P14 &      &       &       &       &       & T3S2  &       &       &       &      &      &      &       &       & T8S1  &       &      & T9S2 & T10S1 &        \\
      P15 &      &       &       &       &       &       & T4S1  &       &       &      &      &      &       &       &       & T8S2  & T9S1 &       &       & T10S2 \\
      P16 &      &       &       &       &       &       &       & T4S2  & T5S1  &      &      &      &       &       &       &       &      & T9S2 & T10S1 &        \\
      \bottomrule
    \end{tabular}
  }
\end{table*}

\section{EVALUATION STUDY QUESTIONNAIRE}

The questionnaire consists of four parts: basic user information, task-related questions, system comparison questions, and semi-structured questions.

\subsection{Basic User Information}

\begin{itemize}
\item Name.
\item Age.
\item Gender.
\item Academic Background.
\item Educational Level.
\item LLMs Usage Frequency (Daily/Weekly/Monthly).
\end{itemize}

\subsection{Task-related Questions}

\begin{table}[htbp]
    \centering
    \caption{Task-related Questions}
    \label{tab:your_label}
    \scriptsize
    \resizebox{\textwidth}{!}{
    \begin{tabular}{l|l|l}
    \toprule
    Task Category & Question & Rating (1-7 points) \\
    \midrule
    C1: Knowledge Exploration & After using this system, how well do you understand this new concept/knowledge point? & \\
    & Please rate it on a scale of 1 to 7, where 1 means no understanding at all and 7 means full understanding. & \\ \hline
    C2: Brainstorming & How well do you feel the system supports your creative work? & \\
 & Please rate on a scale of 1 to 7, where 1 means not at all and 7 means fully support. & \\ \hline
    C3: Product Analysis & When recommending this app to others, are the reasons given by the system logical and organized? & \\
 & Please rate it on a scale of 1 to 7, where 1 means no logic at all and 7 means very clear logic. & \\ \hline
    C4: City Description & Do you think the description of the system is informative? Would others be able to get enough information from the description? & \\
 & Please rate it on a scale of 1 to 7, where 1 is not informative at all and 7 is very informative. & \\
    \bottomrule
    \end{tabular}
    }
\end{table}

\subsection{System Comparison Questions}

\beigin{comment}
\begin{table*}
  \caption{Task-related Questions}
  \label{tab:task_questions}
  \resizebox{\textwidth}{!}{
  \begin{tabular}{l｜l｜l｜l}
    \hline
    & Question & System1 (1-7 points) & System2 (1-7 points) \\
    \hline
    1. & Is the system flexible in terms of operation options in different scenarios? & & \\
       & Please rate it from 1 to 7, with 1 being the least flexible and 7 being the most flexible. & & \\
    \hline
    2. & Does the system allow users to freely adjust and customize content? & & \\
       & Please rate it from 1 to 7, with 1 being the least flexible and 7 being the most flexible. & & \\
    \hline
    3. & Do you feel confident using this product? & & \\
       & Please rate it from 1 to 7, with 1 being very unconfident and 7 being very confident. & & \\
    \hline
    4. & Does it require a lot of learning before using this system? & & \\
       & Please rate it from 1 to 7, with 1 being much learning required and 7 being no learning required. & & \\
    \hline
    5. & Do the system functions and content meet your expectations? & & \\
       & Please rate it from 1 to 7, with 1 being not meeting expectations and 7 being fully meeting expectations. & & \\
    \hline
    6. & How psychologically difficult is it to complete tasks on this system? How much thinking, decision-making, memory, problem solving, etc., does it require? & & \\
       & Please rate it from 1 to 7, with 1 being the most difficult and 7 being the least difficult. & & \\
    \hline
    7. & How urgent is it to complete tasks on this system? Do you feel time-strapped or stressed? & & \\
       & Please rate from 1 to 7, with 1 being the most time pressure and 7 being the least time pressure. & & \\
    \hline
    8. & How satisfied are you with your performance in completing the task on this system? How well or poorly do you feel you completed it? & & \\
       & Please rate from 1 to 7, with 1 being the least satisfied and 7 being the most satisfied. & & \\
    \hline
    9. & What do you think of the results generated by the two systems? Please rate your confidence in the final results. & & \\
       & Please rate from 1 to 7, with 1 being very untrustworthy and 7 being very trustworthy. & & \\
    \hline
  \end{tabular}
  }
\end{table*}
\end{comment}

\subsection{Semi-structured Interview Questions}
